# Supplementary material for: Resource theory of asymmetric distinguishability for quantum channels
Source: arXiv:1907.06306 ancillary file (2019-12-11)
Supplement: Supplementary file 1 [file SDP-duals-channels.pdf]

In this supplementary document, we provide proofs of the various semi-definite programming duals that appear in our paper “Resource theory of asymmetric distinguishability for quantum channels.” We employ the following standard form for the primal semi-definite programs:

$$\inf_{X \geq 0} \{ \text{Tr}[CX] : \Phi(X) \geq D \}, \quad (1)$$

and the dual form is given by

$$\sup_{Y \geq 0} \{ \text{Tr}[DY] : \Phi^\dagger(Y) \leq C \}. \quad (2)$$

If strong duality holds, these two optimizations are equal.

## 1 Normalized diamond distance

The following semi-definite programs were already established in arXiv:0901.4709, but here we give a different proof.

The normalized diamond distance between quantum channels  $\mathcal{N}_{A \rightarrow B}$  and  $\mathcal{M}_{A \rightarrow B}$  can be written as the following semi-definite programs:

$$\frac{1}{2} \|\mathcal{N} - \mathcal{M}\|_\diamond = \sup_{\rho_R, \Omega_{RB} \geq 0} \left\{ \begin{array}{l} \text{Tr}[\Omega_{RB}(\Gamma_{RB}^{\mathcal{N}} - \Gamma_{RB}^{\mathcal{M}})] : \\ \Omega_{RB} \leq \rho_R \otimes I_B, \text{Tr}[\rho_R] = 1 \end{array} \right\} \quad (3)$$

$$= \inf_{\mu, Z_{RB} \geq 0} \left\{ \begin{array}{l} \mu : Z_{RB} \geq \Gamma_{RB}^{\mathcal{N}} - \Gamma_{RB}^{\mathcal{M}}, \\ \mu I_R \geq \text{Tr}_B[Z_{RB}] \end{array} \right\}. \quad (4)$$

The latter expression is equal to

$$\inf_{Z_{RB} \geq 0} \{ \|\text{Tr}_B[Z_{RB}]\|_\infty : Z_{RB} \geq \Gamma_{RB}^{\mathcal{N}} - \Gamma_{RB}^{\mathcal{M}} \}, \quad (5)$$

Employing a well known variational expression for normalized trace distance, consider that

$$\frac{1}{2} \|\mathcal{N} - \mathcal{M}\|_\diamond = \sup_{\psi_{RA}, \Lambda_{RB} \geq 0} \left\{ \begin{array}{l} \text{Tr}[\Lambda_{RB}(\mathcal{N}_{A \rightarrow B} - \mathcal{M}_{A \rightarrow B})(\psi_{RB})] : \\ \Lambda_{RB} \leq I_{RB}, \text{Tr}[\psi_{RA}] = 1, \\ \text{Tr}[\psi_{RA}^2] = 1 \end{array} \right\}, \quad (6)$$

where the constraints  $\psi_{RA} \geq 0$ ,  $\text{Tr}[\psi_{RA}] = 1$ , and  $\text{Tr}[\psi_{RA}^2] = 1$  correspond to  $\psi_{RA}$  being a bipartite pure state. Note that the above is equal to

$$\sup_{\psi_{RA}, \Lambda_{RB} \geq 0} \left\{ \begin{array}{l} \text{Tr}[\Lambda_{RB}(\mathcal{N}_{A \rightarrow B} - \mathcal{M}_{A \rightarrow B})(\psi_{RB})] : \\ \Lambda_{RB} \leq I_{RB}, \psi_R > 0, \\ \text{Tr}[\psi_{RA}] = 1, \text{Tr}[\psi_{RA}^2] = 1 \end{array} \right\}, \quad (7)$$

due to the fact that the set of pure states with reduced state  $\psi_R$  positive definite is dense in the set of all pure states. Any such state  $\psi_{RA}$  can then be written as  $\psi_{RA} = X_R \Gamma_{RA} X_R^\dagger$ , where  $\Gamma_{RA} \equiv |\Gamma\rangle\langle\Gamma|_{RA}$  is defined in terms of

$$|\Gamma\rangle_{RA} := \sum_i |i\rangle_R |i\rangle_A, \quad (8)$$

and  $X_R$  is an arbitrary linear operator such that  $\text{Tr}[X_R^\dagger X_R] = 1$  and  $|X_R| > 0$ . Using this, we find that the objective function can be rewritten as

$$\begin{aligned} & \text{Tr}[\Lambda_{RB}(\mathcal{N}_{A \rightarrow B} - \mathcal{M}_{A \rightarrow B})(X_R \Gamma_{RA} X_R^\dagger)] \\ &= \text{Tr}[X_R^\dagger \Lambda_{RB} X_R (\mathcal{N}_{A \rightarrow B} - \mathcal{M}_{A \rightarrow B})(\Gamma_{RA})] \end{aligned} \quad (9)$$

$$= \text{Tr}[X_R^\dagger \Lambda_{RB} X_R (\Gamma_{RB}^{\mathcal{N}} - \Gamma_{RB}^{\mathcal{M}})]. \quad (10)$$

Now observing the following equivalence:

$$0 \leq \Lambda_{RB} \leq I_{RB} \iff 0 \leq X_R^\dagger \Lambda_{RB} X_R \leq X_R^\dagger X_R \otimes I_B, \quad (11)$$

and defining  $\Omega_{RB} := X_R^\dagger \Lambda_{RB} X_R$ , the optimization in (7) is equal to the following one:

$$\sup_{\rho_R, \Omega_{RB} \geq 0} \left\{ \begin{array}{l} \text{Tr}[\Omega_{RB}(\Gamma_{RB}^{\mathcal{N}} - \Gamma_{RB}^{\mathcal{M}})] : \\ \Omega_{RB} \leq \rho_R \otimes I_B, \\ \rho_R > 0, \text{Tr}[\rho_R] = 1 \end{array} \right\}, \quad (12)$$

giving the equality in (3), after again using the fact that the set of operators  $\rho_R$  satisfying  $\rho_R > 0$  is dense in the set of those satisfying  $\rho_R \geq 0$ .

Now setting

$$Y := \begin{bmatrix} \Omega_{RB} & 0 \\ 0 & \rho_R \end{bmatrix}, \quad (13)$$

$$D := \begin{bmatrix} \Gamma_{RB}^{\mathcal{N}} - \Gamma_{RB}^{\mathcal{M}} & 0 \\ 0 & 0 \end{bmatrix}, \quad (14)$$

$$\Phi^\dagger(Y) := \begin{bmatrix} \Omega_{RB} - \rho_R \otimes I_B & 0 & 0 \\ 0 & \text{Tr}[\rho_R] & 0 \\ 0 & 0 & -\text{Tr}[\rho_R] \end{bmatrix}, \quad (15)$$

$$C := \begin{bmatrix} 0 & 0 & 0 \\ 0 & 1 & 0 \\ 0 & 0 & -1 \end{bmatrix}, \quad (16)$$

we find that (3) is now in the standard form

$$\sup_{Y \geq 0} \left\{ \text{Tr}[DY] : \Phi^\dagger(Y) \leq C \right\}. \quad (17)$$

The dual map  $\Phi$  is found from  $\Phi^\dagger$  by solving for  $\Phi$  in

$$\text{Tr}[\Phi^\dagger(Y)Z] = \text{Tr}[Y\Phi(Z)], \quad (18)$$

with

$$Z := \begin{bmatrix} Z_{RB} & 0 & 0 \\ 0 & \mu_1 & 0 \\ 0 & 0 & \mu_2 \end{bmatrix}, \quad (19)$$

from which we find that

$$\text{Tr}[\Phi^\dagger(Y)Z] = \text{Tr}[(\Omega_{RB} - \rho_R \otimes I_B)Z_{RB}] + \text{Tr}[\rho_R]\mu_1 - \text{Tr}[\rho_R]\mu_2 \quad (20)$$

$$= \text{Tr}[\Omega_{RB}Z_{RB}^1] + \text{Tr}[\rho_R((\mu_1 - \mu_2)I_R - \text{Tr}_B[Z_{RB}])]. \quad (21)$$

Then we conclude that

$$\Phi(Z) = \begin{bmatrix} Z_{RB} & 0 \\ 0 & (\mu_1 - \mu_2)I_R - \text{Tr}_B[Z_{RB}] \end{bmatrix}. \quad (22)$$

The standard form of the dual is given by

$$\inf_{Z \geq 0} \{ \text{Tr}[CZ] : \Phi(Z) \geq D \}, \quad (23)$$

which becomes

$$\inf_{\mu_1, \mu_2, Z_{RB} \geq 0} \left\{ \begin{array}{l} \mu_1 - \mu_2 : \\ Z_{RB} \geq \Gamma_{RB}^{\mathcal{N}} - \Gamma_{RB}^{\mathcal{M}}, \\ (\mu_1 - \mu_2)I_R \geq \text{Tr}_B[Z_{RB}]. \end{array} \right\}. \quad (24)$$

First note that the variables  $\mu_1$  and  $\mu_2$  always appear together above as  $\mu_1 - \mu_2$ , and so can be reduced to a single real variable  $\mu \in \mathbb{R}$ . However, the condition  $\mu I_R \geq \text{Tr}_B[Z_{RB}]$ , implies that  $\mu \geq 0$ . Thus, the optimization can be simplified to

$$\inf_{\mu, Z_{RB} \geq 0} \left\{ \begin{array}{l} \mu : Z_{RB} \geq \Gamma_{RB}^{\mathcal{N}} - \Gamma_{RB}^{\mathcal{M}}, \\ \mu I_R \geq \text{Tr}_B[Z_{RB}] \end{array} \right\}, \quad (25)$$

which is equal to

$$\inf_{Z_{RB} \geq 0} \{ \|\text{Tr}_B[Z_{RB}]\|_\infty : Z_{RB} \geq \Gamma_{RB}^{\mathcal{N}} - \Gamma_{RB}^{\mathcal{M}} \}, \quad (26)$$

by the definition of the Schatten  $\infty$ -norm for positive semi-definite operators.

Strong duality holds because the choice  $Z_{RB} = \Gamma_{RB}^{\mathcal{N}} - \Gamma_{RB}^{\mathcal{M}} + \delta I_{RB}$  is strictly feasible for  $\delta > 0$ .

## 2 Approximate channel box transformation problem

The approximate channel box transformation problem is given by the following optimization:

$$\inf_{Z_{CD}, \Gamma_{CBAD}^\Theta \geq 0} \|\text{Tr}_D[Z_{CD}]\|_\infty, \quad (27)$$

subject to

$$\begin{aligned} Z_{CD} &\geq \Gamma_{CD}^\mathcal{K} - \text{Tr}_{AB}[(\Gamma_{AB}^\mathcal{N})^T \Gamma_{CBAD}^\Theta], \\ \Gamma_{CD}^\mathcal{L} &= \text{Tr}_{AB}[(\Gamma_{AB}^\mathcal{M})^T \Gamma_{CBAD}^\Theta], \\ \Gamma_{CB}^\Theta &= I_{CB}, \\ \Gamma_{CBA}^\Theta &= \Gamma_{CA}^\Theta \otimes \pi_B, \end{aligned} \quad (28)$$

Consider that this is equal to

$$\inf_{\mu, Z_{CD}, \Gamma_{CBAD}^\Theta \geq 0} \mu, \quad (29)$$

subject to

$$\begin{aligned} \mu I_C &\geq \text{Tr}_D[Z_{CD}], \quad Z_{CD} \geq \Gamma_{CD}^\mathcal{K} - \text{Tr}_{AB}[(\Gamma_{AB}^\mathcal{N})^T \Gamma_{CBAD}^\Theta], \\ \Gamma_{CD}^\mathcal{L} &= \text{Tr}_{AB}[(\Gamma_{AB}^\mathcal{M})^T \Gamma_{CBAD}^\Theta], \\ \Gamma_{CB}^\Theta &= I_{CB}, \quad \Gamma_{CBA}^\Theta = \Gamma_{CA}^\Theta \otimes \pi_B, \end{aligned}$$

An SDP in standard form can be written as

$$\inf_{X \geq 0} \{\text{Tr}[XC] : \Phi(X) \geq D\}. \quad (30)$$

So we identify

$$X = \begin{bmatrix} \mu & 0 & 0 \\ 0 & Z_{CD} & 0 \\ 0 & 0 & \Gamma_{CBAD}^\Theta \end{bmatrix}, \quad (31)$$

$$C = \begin{bmatrix} 1 & 0 & 0 \\ 0 & 0 & 0 \\ 0 & 0 & 0 \end{bmatrix}, \quad (32)$$

$$\Phi(X) = \text{diag} \left( \begin{bmatrix} \mu I_C - \text{Tr}_D[Z_{CD}] \\ Z_{CD} + \text{Tr}_{AB}[(\Gamma_{AB}^{\mathcal{N}})^T \Gamma_{CBAD}^{\Theta}] \\ \text{Tr}_{AB}[(\Gamma_{AB}^{\mathcal{M}})^T \Gamma_{CBAD}^{\Theta}] \\ -\text{Tr}_{AB}[(\Gamma_{AB}^{\mathcal{M}})^T \Gamma_{CBAD}^{\Theta}] \\ \Gamma_{CB}^{\Theta} \\ -\Gamma_{CB}^{\Theta} \\ \Gamma_{CBA}^{\Theta} - \Gamma_{CA}^{\Theta} \otimes \pi_B \\ -\Gamma_{CBA}^{\Theta} + \Gamma_{CA}^{\Theta} \otimes \pi_B \end{bmatrix} \right) \quad (33)$$

$$D = \text{diag} \left( \begin{bmatrix} 0 \\ \Gamma_{CD}^{\mathcal{K}} \\ \Gamma_{CD}^{\mathcal{L}} \\ -\Gamma_{CD}^{\mathcal{L}} \\ I_{CB} \\ -I_{CB} \\ 0 \\ 0 \end{bmatrix} \right) \quad (34)$$

The dual SDP is given by

$$\sup_{Y \geq 0} \left\{ \text{Tr}[DY] : \Phi^\dagger(Y) \leq C \right\}. \quad (35)$$

So we need to compute  $\Phi^\dagger$  from

$$\text{Tr}[\Phi(X)Y] = \text{Tr}[X\Phi^\dagger(Y)]. \quad (36)$$

Taking  $Y$  to be

$$Y = \text{diag} \left( \begin{bmatrix} Y_C^1 \\ Y_{CD}^2 \\ Y_{CD}^3 \\ Y_{CD}^4 \\ Y_{CB}^5 \\ Y_{CB}^6 \\ Y_{CBA}^7 \\ Y_{CBA}^8 \end{bmatrix} \right), \quad (37)$$

we find that

$$\begin{aligned}
& \text{Tr}[\Phi(X)Y] \\
&= \text{Tr}[(\mu I_C - \text{Tr}_D[Z_{CD}]) Y_C^1] + \text{Tr}[(Z_{CD} + \text{Tr}_{AB}[(\Gamma_{AB}^{\mathcal{N}})^T \Gamma_{CBAD}^{\Theta}]) Y_{CD}^2] \\
&+ \text{Tr}[(\text{Tr}_{AB}[(\Gamma_{AB}^{\mathcal{M}})^T \Gamma_{CBAD}^{\Theta}]) (Y_{CD}^3 - Y_{CD}^4)] + \text{Tr}[\Gamma_{CB}^{\Theta} (Y_{CB}^5 - Y_{CB}^6)] \\
&+ \text{Tr}[(\Gamma_{CBA}^{\Theta} - \Gamma_{CA}^{\Theta} \otimes \pi_B) (Y_{CBA}^7 - Y_{CBA}^8)] \\
&= \mu \text{Tr}[Y_C^1] + \text{Tr}[Z_{CD} (Y_{CD}^2 - Y_C^1 \otimes I_D)] \\
&+ \text{Tr} \left[ \Gamma_{CBAD}^{\Theta} \begin{pmatrix} Y_{CD}^2 \otimes (\Gamma_{AB}^{\mathcal{N}})^T + (Y_{CD}^3 - Y_{CD}^4) \otimes (\Gamma_{AB}^{\mathcal{M}})^T + (Y_{CB}^5 - Y_{CB}^6) \otimes I_{AD} \\ + (Y_{CBA}^7 - Y_{CBA}^8) \otimes I_D - I_{BD} \otimes \text{Tr}_B[(Y_{CBA}^7 - Y_{CBA}^8)]/|B| \end{pmatrix} \right] \\
&\hspace{15cm} (39)
\end{aligned}$$

So this means that

$$\Phi^\dagger(Y) = \text{diag} \left( \begin{bmatrix} \text{Tr}[Y_C^1] \\ Y_{CD}^2 - Y_C^1 \otimes I_D \\ \Upsilon_{CDAB} \end{bmatrix} \right), \quad (40)$$

where

$$\begin{aligned}
\Upsilon_{CDAB} &:= Y_{CD}^2 \otimes (\Gamma_{AB}^{\mathcal{N}})^T + (Y_{CD}^3 - Y_{CD}^4) \otimes (\Gamma_{AB}^{\mathcal{M}})^T + (Y_{CB}^5 - Y_{CB}^6) \otimes I_{AD} \\
&+ (Y_{CBA}^7 - Y_{CBA}^8) \otimes I_D - I_{BD} \otimes \text{Tr}_B[(Y_{CBA}^7 - Y_{CBA}^8)]/|B|. \quad (41)
\end{aligned}$$

So then the dual is given by

$$\begin{aligned}
& \sup_{Y \geq 0} \left\{ \text{Tr}[DY] : \Phi^\dagger(Y) \leq C \right\} \\
&= \sup_{Y \geq 0} \left\{ \begin{array}{l} \text{Tr}[\Gamma_{CD}^{\mathcal{K}} Y_{CD}^2] + \text{Tr}[\Gamma_{CD}^{\mathcal{L}} (Y_{CD}^3 - Y_{CD}^4)] + \text{Tr}[Y_{CB}^5 - Y_{CB}^6] : \\ \text{Tr}[Y_C^1] \leq 1, Y_{CD}^2 \leq Y_C^1 \otimes I_D, \\ Y_{CD}^2 \otimes (\Gamma_{AB}^{\mathcal{N}})^T + (Y_{CD}^3 - Y_{CD}^4) \otimes (\Gamma_{AB}^{\mathcal{M}})^T + (Y_{CB}^5 - Y_{CB}^6) \otimes I_{AD} \\ + (Y_{CBA}^7 - Y_{CBA}^8) \otimes I_D - I_{BD} \otimes \text{Tr}_B[(Y_{CBA}^7 - Y_{CBA}^8)]/|B| \leq 0. \end{array} \right\} \\
&\hspace{15cm} (42)
\end{aligned}$$

We can now identify  $W_{CD} := Y_{CD}^3 - Y_{CD}^4$  as Hermitian,  $S_{CB} := Y_{CB}^5 - Y_{CB}^6$  as Hermitian,  $L_{CBA} := Y_{CBA}^7 - Y_{CBA}^8$  as Hermitian. Then the above simplifies to

$$\sup_{\substack{Y_{CD}, M_C \geq 0, \\ W_{CD}, S_{CB}, L_{CBA} \in \text{Herm}}} \left\{ \begin{array}{l} \text{Tr}[\Gamma_{CD}^{\mathcal{K}} Y_{CD}] + \text{Tr}[\Gamma_{CD}^{\mathcal{L}} W_{CD}] + \text{Tr}[S_{CB}] : \\ \text{Tr}[M_C] \leq 1, Y_{CD} \leq M_C \otimes I_D, \\ Y_{CD} \otimes (\Gamma_{AB}^{\mathcal{N}})^T + W_{CD} \otimes (\Gamma_{AB}^{\mathcal{M}})^T + S_{CB} \otimes I_{AD} \\ + L_{CBA} \otimes I_D - I_{BD} \otimes \text{Tr}_B[L_{CBA}]/|B| \leq 0. \end{array} \right\} \quad (43)$$

### 3 Smooth channel min-relative entropy

The smooth channel min-relative entropy is given by the following optimization:

$$\inf_{\rho_R, \Omega_{RB} \geq 0} \left\{ \begin{array}{l} \text{Tr}[\Omega_{RB} \Gamma_{RB}^{\mathcal{M}}] : \\ \text{Tr}[\Omega_{RB} \Gamma_{RB}^{\mathcal{N}}] \geq 1 - \varepsilon, \\ \Omega_{RB} \leq \rho_R \otimes I_B, \text{Tr}[\rho_R] = 1 \end{array} \right\}. \quad (44)$$

The standard form is given by

$$\inf_{X \geq 0} \{ \text{Tr}[XC] : \Phi(X) \geq D \}, \quad (45)$$

with

$$X = \begin{bmatrix} \Omega_{RB} & 0 \\ 0 & \rho_R \end{bmatrix}, \quad (46)$$

$$C = \begin{bmatrix} \Gamma_{RB}^{\mathcal{M}} & 0 \\ 0 & 0 \end{bmatrix}, \quad (47)$$

$$\Phi(X) = \begin{bmatrix} \text{Tr}[\Omega_{RB} \Gamma_{RB}^{\mathcal{N}}] & 0 & 0 & 0 \\ 0 & \rho_R \otimes I_B - \Omega_{RB} & 0 & 0 \\ 0 & 0 & \text{Tr}[\rho_R] & 0 \\ 0 & 0 & 0 & -\text{Tr}[\rho_R] \end{bmatrix}, \quad (48)$$

$$D = \begin{bmatrix} 1 - \varepsilon & 0 & 0 & 0 \\ 0 & 0 & 0 & 0 \\ 0 & 0 & 1 & 0 \\ 0 & 0 & 0 & -1 \end{bmatrix}. \quad (49)$$

Then the adjoint of  $\Phi$  is given by

$$\text{Tr}[\Phi(X)Y] = \text{Tr}[X\Phi^\dagger(Y)], \quad (50)$$

where

$$Y = \begin{bmatrix} \mu_1 & 0 & 0 & 0 \\ 0 & Y_{RB} & 0 & 0 \\ 0 & 0 & \mu_2 & 0 \\ 0 & 0 & 0 & \mu_3 \end{bmatrix}. \quad (51)$$

Then we find that

$$\begin{aligned} & \text{Tr}[\Phi(X)Y] \\ &= \text{Tr} \left[ \begin{bmatrix} \text{Tr}[\Omega_{RB}\Gamma_{RB}^{\mathcal{N}}] & 0 & 0 & 0 \\ 0 & \rho_R \otimes I_B - \Omega_{RB} & 0 & 0 \\ 0 & 0 & \text{Tr}[\rho_R] & 0 \\ 0 & 0 & 0 & -\text{Tr}[\rho_R] \end{bmatrix} \begin{bmatrix} \mu_1 & 0 & 0 & 0 \\ 0 & Y_{RB} & 0 & 0 \\ 0 & 0 & \mu_2 & 0 \\ 0 & 0 & 0 & \mu_3 \end{bmatrix} \right] \end{aligned} \quad (52)$$

$$= \mu_1 \text{Tr}[\Omega_{RB}\Gamma_{RB}^{\mathcal{N}}] + \text{Tr}[(\rho_R \otimes I_B - \Omega_{RB}) Y_{RB}] + (\mu_2 - \mu_3) \text{Tr}[\rho_R] \quad (53)$$

$$= \text{Tr}[\Omega_{RB} (\mu_1 \Gamma_{RB}^{\mathcal{N}} - Y_{RB})] + \text{Tr}[\rho_R [(\mu_2 - \mu_3) I_R + \text{Tr}_B[Y_{RB}]]], \quad (54)$$

implying that

$$\Phi^\dagger(Y) = \begin{bmatrix} \mu_1 \Gamma_{RB}^{\mathcal{N}} - Y_{RB} & 0 \\ 0 & (\mu_2 - \mu_3) I_R + \text{Tr}_B[Y_{RB}] \end{bmatrix}. \quad (55)$$

The dual is then given by

$$\sup_{Y \geq 0} \left\{ \text{Tr}[YD] : \Phi^\dagger(Y) \leq C \right\}. \quad (56)$$

By plugging in, we find that the dual is given by

$$\sup_{\mu_1, \mu_2, \mu_3, Y_{RB} \geq 0} \left\{ \begin{array}{l} (1 - \varepsilon) \mu_1 + \mu_2 - \mu_3 : \\ \mu_1 \Gamma_{RB}^{\mathcal{N}} - Y_{RB} \leq \Gamma_{RB}^{\mathcal{M}}, \\ \text{Tr}_B[Y_{RB}] \leq -(\mu_2 - \mu_3) I_R \end{array} \right\}. \quad (57)$$

We can then simplify this as

$$\begin{aligned} & \sup_{\lambda, Y_{RB} \geq 0, \mu \in \mathbb{R}} \left\{ \begin{array}{l} (1 - \varepsilon) \lambda - \mu : \\ \lambda \Gamma_{RB}^{\mathcal{N}} \leq \Gamma_{RB}^{\mathcal{M}} + Y_{RB}, \\ \text{Tr}_B[Y_{RB}] \leq \mu I_R \end{array} \right\} \\ &= \sup_{\lambda, \mu, Y_{RB} \geq 0} \left\{ \begin{array}{l} (1 - \varepsilon) \lambda - \mu : \\ \lambda \Gamma_{RB}^{\mathcal{N}} \leq \Gamma_{RB}^{\mathcal{M}} + Y_{RB}, \\ \text{Tr}_B[Y_{RB}] \leq \mu I_R \end{array} \right\} \end{aligned} \quad (58)$$

## 4 Smooth channel max-relative entropy

The SDP formulation of the channel smooth max-relative entropy is given by

$$\inf_{\substack{\lambda, Z_{RB}, \\ W_{RB} \geq 0}} \left\{ \begin{array}{l} \lambda : \\ W_{RB} \leq \lambda \Gamma_{RB}^{\mathcal{M}}, \text{Tr}_B[W_{RB}] = I_R \\ \varepsilon I_R \geq \text{Tr}_B[Z_{RB}], \\ Z_{RB} \geq \Gamma_{RB}^{\mathcal{N}} - W_{RB} \end{array} \right\}. \quad (59)$$

The standard form is given by

$$\inf_{X \geq 0} \{ \text{Tr}[XC] : \Phi(X) \geq D \}. \quad (60)$$

with

$$X = \begin{bmatrix} \lambda & 0 & 0 \\ 0 & Z_{RB} & 0 \\ 0 & 0 & W_{RB} \end{bmatrix}, \quad (61)$$

$$C = \begin{bmatrix} 1 & 0 & 0 \\ 0 & 0 & 0 \\ 0 & 0 & 0 \end{bmatrix}, \quad (62)$$

$$\Phi(X) = \begin{bmatrix} \lambda \Gamma_{RB}^{\mathcal{M}} - W_{RB} & 0 & 0 & 0 & 0 \\ 0 & \text{Tr}_B W_{RB} & 0 & 0 & 0 \\ 0 & 0 & -\text{Tr}_B W_{RB} & 0 & 0 \\ 0 & 0 & 0 & -\text{Tr}_B [Z_{RB}] & 0 \\ 0 & 0 & 0 & 0 & Z_{RB} + W_{RB} \end{bmatrix}, \quad (63)$$

$$D = \begin{bmatrix} 0 & 0 & 0 & 0 & 0 \\ 0 & I_R & 0 & 0 & 0 \\ 0 & 0 & -I_R & 0 & 0 \\ 0 & 0 & 0 & -\varepsilon I_R & 0 \\ 0 & 0 & 0 & 0 & \Gamma_{RB}^{\mathcal{N}} \end{bmatrix}. \quad (64)$$

To figure out the dual map  $\Phi^\dagger$ , we consider that

$$\text{Tr}[\Phi(X)Y] = \text{Tr}[X\Phi^\dagger(Y)], \quad (65)$$

where

$$Y = \begin{bmatrix} Y_{RB}^1 & 0 & 0 & 0 & 0 \\ 0 & Y_R^2 & 0 & 0 & 0 \\ 0 & 0 & Y_R^3 & 0 & 0 \\ 0 & 0 & 0 & Y_R^4 & 0 \\ 0 & 0 & 0 & 0 & Y_{RB}^5 \end{bmatrix}. \quad (66)$$

Then

$$\begin{aligned} \text{Tr}[\Phi(X)Y] &= \text{Tr}[(\lambda \Gamma_{RB}^{\mathcal{M}} - W_{RB}) Y_{RB}^1] + \text{Tr}[\text{Tr}_B [W_{RB}] (Y_R^2 - Y_R^3)] \\ &\quad - \text{Tr}[\text{Tr}_B [Z_{RB}] Y_R^4] + \text{Tr}[(Z_{RB} + W_{RB}) Y_{RB}^5] \end{aligned} \quad (67)$$

$$\begin{aligned} &= \lambda \text{Tr}[\Gamma_{RB}^{\mathcal{M}} Y_{RB}^1] \\ &\quad + \text{Tr}[Z_{RB} (Y_{RB}^5 - Y_R^4 \otimes I_B)] \\ &\quad + \text{Tr}[W_{RB} (-Y_{RB}^1 + (Y_R^2 - Y_R^3) \otimes I_B + Y_{RB}^5)]. \end{aligned} \quad (68)$$

So we see that

$$\Phi^\dagger(Y) = \begin{bmatrix} \text{Tr}[\Gamma_{RB}^{\mathcal{M}} Y_{RB}^1] & 0 & 0 \\ 0 & Y_{RB}^5 - Y_R^4 \otimes I_B & 0 \\ 0 & 0 & -Y_{RB}^1 + (Y_R^2 - Y_R^3) \otimes I_B + Y_{RB}^5 \end{bmatrix} \quad (69)$$

The dual is then given by

$$\sup_{Y \geq 0} \left\{ \text{Tr}[YD] : \Phi^\dagger(Y) \leq C \right\}. \quad (70)$$

Plugging in, we find that the dual is

$$\begin{aligned} & \sup_{Y_{RB}^1, Y_R^2, Y_R^3, Y_R^4, Y_{RB}^5 \geq 0} \left\{ \begin{array}{l} \text{Tr}[Y_R^2 - Y_R^3] - \varepsilon \text{Tr}[Y_R^4] + \text{Tr}[Y_{RB}^5 \Gamma_{RB}^{\mathcal{N}}] : \\ \text{Tr}[\Gamma_{RB}^{\mathcal{M}} Y_{RB}^1] \leq 1, \\ Y_{RB}^5 - Y_R^4 \otimes I_B \leq 0, \\ -Y_{RB}^1 + (Y_R^2 - Y_R^3) \otimes I_B + Y_{RB}^5 \leq 0 \end{array} \right\} \\ &= \sup_{\substack{Y_{RB}^1, Y_R^4, Y_{RB}^5 \geq 0, \\ Z_R \in \text{Herm}}} \left\{ \begin{array}{l} \text{Tr}[Z_R] - \varepsilon \text{Tr}[Y_R^4] + \text{Tr}[Y_{RB}^5 \Gamma_{RB}^{\mathcal{N}}] : \\ \text{Tr}[\Gamma_{RB}^{\mathcal{M}} Y_{RB}^1] \leq 1, \\ Y_{RB}^5 - Y_R^4 \otimes I_B \leq 0, \\ -Y_{RB}^1 + Z_R \otimes I_B + Y_{RB}^5 \leq 0 \end{array} \right\} \\ &= \sup_{\substack{Y_{RB}^1, Y_R^4, Y_{RB}^5 \geq 0, \\ Z_R \in \text{Herm}}} \left\{ \begin{array}{l} \text{Tr}[Z_R] - \varepsilon \text{Tr}[Y_R^4] + \text{Tr}[Y_{RB}^5 \Gamma_{RB}^{\mathcal{N}}] : \\ \text{Tr}[\Gamma_{RB}^{\mathcal{M}} Y_{RB}^1] \leq 1, \\ Y_{RB}^5 \leq Y_R^4 \otimes I_B, \\ Z_R \otimes I_B + Y_{RB}^5 \leq Y_{RB}^1 \end{array} \right\}. \end{aligned}$$
